# Supplementary material for: Time Crystals from single-molecule magnet arrays
Source: arXiv:2409.10816 ancillary file (2024-09-17)
Supplement: Supplementary file 1 [file SI_for_publication.pdf]

# Supporting Information: Time Crystals from single-molecule magnet arrays

Subhajit Sarkar[*,†] and Yonatan Dubi[*,¶]

†*Department of Physics and Nanotechnology, SRM Institute of Science and Technology Kattankulathur-603 203, India.*

‡*Institute of Theoretical Physics, Jagiellonian University, Lojasiewicza 11, 30-348, Krakow, Poland,*

¶*Department of Chemistry, Ben-Gurion University of the Negev, Beer Sheva 84105, Israel,*

§*Ilse Katz Center for Nanoscale Science and Technology, Ben-Gurion University of the Negev, Beer Sheva 84105, Israel.*

E-mail: sbhjt72@gmail.com,subhajis@srmist.edu.in; jdubi@bgu.ac.il

**Abstract**

In this supporting information, we provide all the necessary details of the calculations and extra plots to substantiate our claims in the main paper.

## System size dependence of the DTC frequency

In the main text, we have shown how DTC appears in the oscillation of the average magnetization and concluded that for large values of both $N$ and $S$ (theoretically as $N \to \infty$ and $S \to \infty$), the DTC oscillation can maintain its robustness indefinitely. To illustrate this further we plot the discrete Fourier transform, $\Phi[\langle S_j^z(t) \rangle](f)$ in Fig. 1 as a function of $f/\omega$ for different values of $J$ being, (aj) $0.001D$, (bj) $0.01D$, (cj) $0.1D$, (dj) $D$, and, (ej) $10D$,

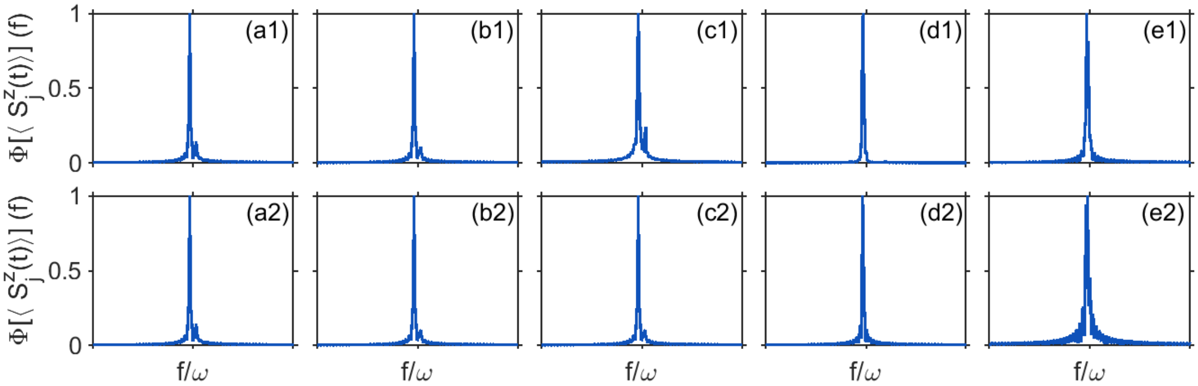


Figure 1: Plots of DFT of onsite magnetization $\Phi[\langle S^z_j(t)\rangle](f)$ as a function of $f/\omega$ for different values of $J$ being, (aj) $0.001D$, (bj) $0.01D$, (cj) $0.1D$, (dj) $D$, and , (ej) $10D$, with $j = 1$ and $j = 2$ corresponding to $N = 3$ and $N = 5$, respectively.

with $j = 1$ and $j = 2$ corresponding to $N = 3$ and $N = 5$, respectively, corresponding to $S = 1$. This indicates that the DTC frequency remains unaffected by increasing the chain size.

# Choice of the initial states

To elucidate why the exchange coupling doesn't precisely dictate the value of the discrete time crystal (DTC) frequency, we must commence our analysis from varied initial density matrices, denoted by $\rho_{in}$. For these matrices, the spin configuration is expressed as $\langle S^z_j\rangle_{in} = Tr[S^z_j \rho_{in}]$. We can conveniently categorize these initial states into a non-synchronized state, implying different local magnetizations at each site, and a synchronized state that exhibits identical magnetization across all sites.

In situations where the initial state is not synchronized across each site corresponding to $\langle S^z_j\rangle_{in} = 0, 1, 0, 1$ and $1, 0, 1, 0$, the weakly interacting chain (with $J$ equating to $0.1D$) displays oscillation that stems from the energy levels of the individual single-molecule magnets (SMMs). This phenomenon is observable in the Discrete Fourier Transform (DFT) of on-site magnetization in Fig. 2, which reveals two frequencies indicative of a weaker $J$ value. Conversely, for stronger $J$ values, a non-synchronized initial state leads to noisy oscillation

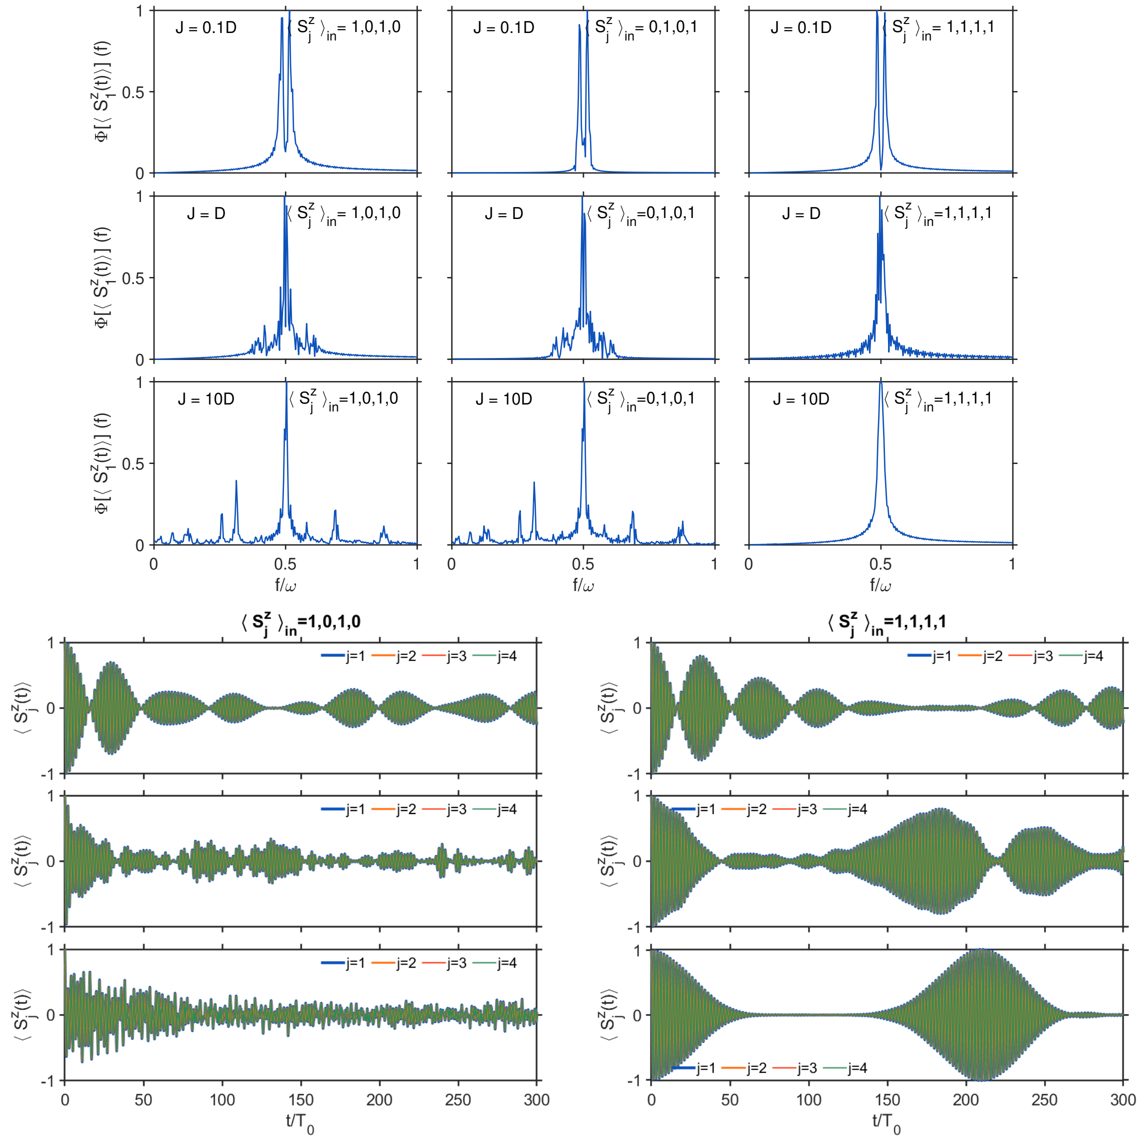


Figure 2: Upper panel: Plots of the discrete Fourier transform of the oscillation of on-site magnetization $\langle S_j^z \rangle$ for different initial states with configuration indicated by the on-site magnetization; bottom left and right: Plots of the oscillation of on-site magnetization $\langle S_j^z \rangle$ (for a 4-site chain) corresponding to the initial state with configuration $\langle S_j^z \rangle = 1;0;1;0$ and $1;1;1;1$, respectively, with increasing values of exchange coupling $J = 0.1D$, $D$ and $10D$ from top to bottom, respectively.

seen in Fig. 2, as evidenced by the DFTs corresponding to $J = D$ and $J = 10D$ scenarios.

When the initial state is synchronized at each site corresponding to $\langle S_j^z \rangle_{in} = 1, 1, 1, 1$, the weakly interacting chain (once again with $J = 0.1D$) keeps demonstrating oscillation originating from individual SMMs, alongside two frequencies in the DFT of the on-site magnetization, a marker of weaker $J$. However, in cases of stronger $J$ ($J = D$ and $J = 10D$), these two frequencies merge to yield a singular DTC frequency, seen in Fig. 2. This union results in a $J$-independent DTC oscillation.

The above-outlined physical interpretation is further corroborated by the oscillation of on-site magnetization. Importantly, despite an initial state of non-synchronization, each site experiences synchronized oscillation across all cases, culminating in quantum synchronization.

# Static Hamiltonian in the rotated frame

We consider the Spin-S Hamiltonian

$$\mathcal{H} = \mathcal{H}_0 + \mathbf{B}(t) \cdot \sum_j \mathbf{S}_j = -J \sum_j \mathbf{S}_j \cdot \mathbf{S}_{j+1} - \sum_j D(S_j^z)^2 + \mathbf{B}(t) \cdot \sum_j \mathbf{S}_j, \qquad (1)$$

in a time-dependent external magnetic field

$$\mathcal{H}_{ext}(t) = \mathbf{B}(t) \cdot \sum_j \mathbf{S}_j = \sum_j \left[ \frac{B}{2} \left( S_j^+ e^{-i\omega t} + S_j^- e^{i\omega t} \right) + B' S_j^z \right]. \qquad (2)$$

We can use an unitary transformation $\mathcal{U}(t) = e^{i\omega t \sum_j (1 - S_j^z)}$. The static part of the Hamiltonian satisfies $\left[ \mathcal{H}_0, \sum_k S_k^z \right] = 0$ because the total magnetization is a conserved quantity thereby, $\mathcal{U}^\dagger(t)\mathcal{H}_0\mathcal{U}(t) = \mathcal{H}_0$. However, it is easy to show that $\mathcal{U}^\dagger(t)\mathcal{H}_{ext}\mathcal{U}(t) - i\mathcal{U}^\dagger(t)\frac{\partial \mathcal{U}(t)}{\partial t} = (B, 0, B' - \omega) \cdot \sum_j \mathbf{S}_j$. With the choice of $B' - \omega = 0$, our final Floquet Hamiltonian is given by, $\mathcal{H}_F = -J \sum_j \mathbf{S}_j \cdot \mathbf{S}_{j+1} + \sum_j \left[ -D(S_j^z)^2 + BS_j^x \right]$ which we used in the main text to

analyze the origin of the DTC frequency.

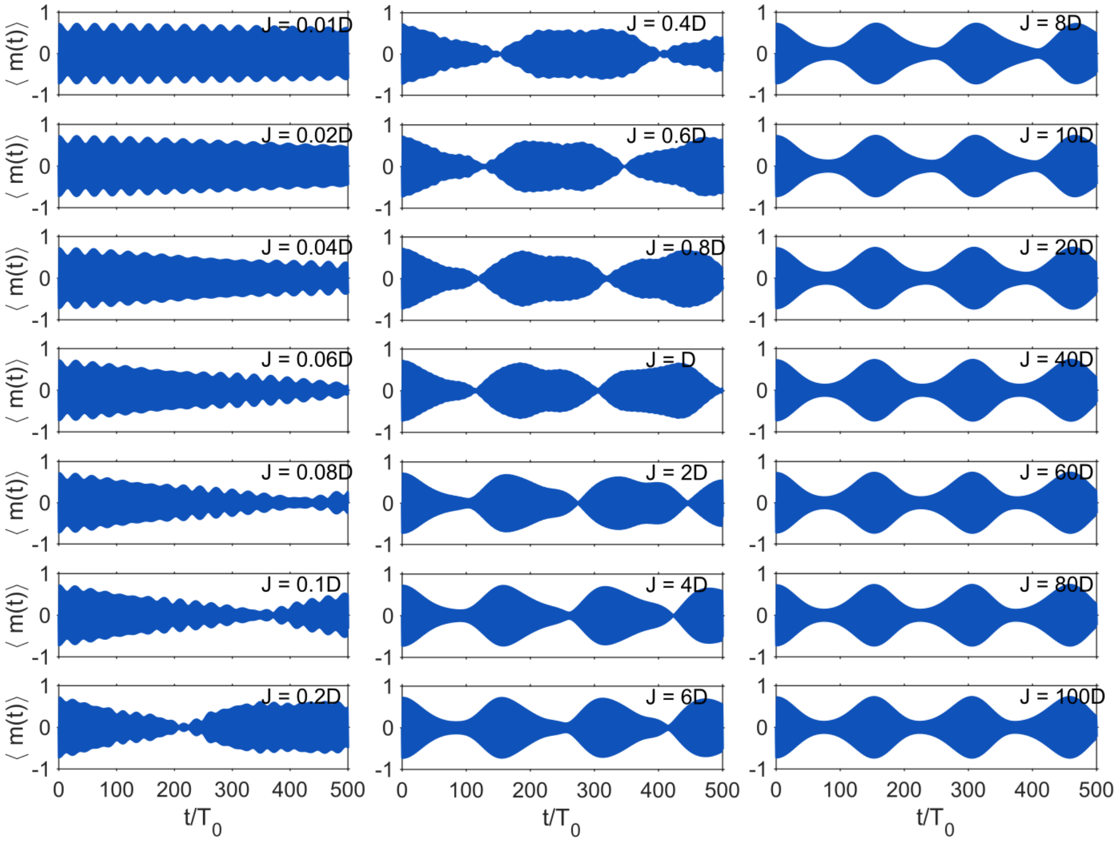


Figure 3: Plots of average magnetization $\langle m(t)\rangle$ as a function of $t/T_0$ up to 500 periods of external drive for different values of $J$ ranging from $0.01D$ to $100D$.

In the main text, we reported that the pulse profile of the magnetization dynamics originates from the exchange interaction. To substantiate our claim further, we plot the dynamics of the average magnetization $\langle m(t)\rangle$ as a function of $t/T_0$ up to 500 periods of external drive for different values of $J$ ranging from $0.01D$ to $100D$ in Fig. 3. This implies a few important features, (1) the DTC oscillation persists for a long time perhaps enough to observe in the experiment, (2) with increasing the value of the exchange coupling the envelope of the oscillation changes and a pulsating character starts to appear, (3) from $J = 10D$ and higher the pulsating character of the oscillation remains unchanged indicating the many-body origin of the effect.

Here we further elaborate on our choice of $B' - \omega = 0$. Fig. 4 plots the sub-harmonic

oscillation when $B' = \omega/2$ in Fig. 4(a) and when $B' = 3\omega/2$ in Fig. 4(c). These plots clearly show that the DTC response oscillates around a net mean magnetization defined as $\frac{1}{T_{DTC}} \int_0^{T_{DTC}} dt \langle S_j^z(t) \rangle \neq 0$ over one period of the DTC oscillation. For $B' = \omega$ and $B' = 3\omega/2$ the mean magnetizations are negative and positive, respectively. The corresponding DFTs are plotted in Fig. 4(b) and (d), respectively, where, beside the sub-harmonic frequency, a zero frequency component corresponding to the DFT of $\langle S_j^z(t) \rangle$ indicates the existence of a non-zero constant component in the DTC oscillation.

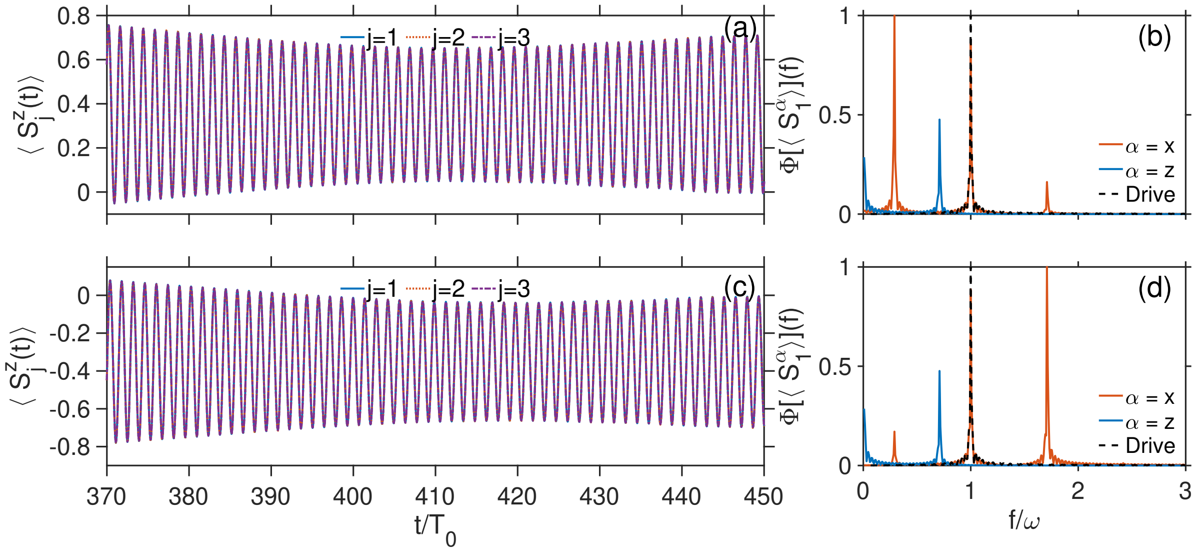


Figure 4: Plot of on-site magnetization $\langle S_j^z(t) \rangle$ and the corresponding DFT, (a) and (b) for $B' = \omega/2$, and (c) and (d) for $B' = 3\omega/2$ for $N = 3$ with $J = 10D$. In (b) and (d) the black dashed line represents the DTF of the periodic drive.

# Mechanism of the DTC and difference from the Rabi oscillations

From our study, initial observations indicate that when the coupling constant $J = 0$, the dominant frequency of system oscillations appears unchanged, suggesting similarities to Rabi oscillations seen in isolated SMMs. This might initially imply that the observed behavior in DTCs merely extends these single-molecule phenomena. However, further examination

reveals a more complex scenario when molecules are coupled.

By coupling Single-Molecule Magnets (SMMs) via Heisenberg exchange interactions, an extra energy scale, the exchange coupling, $J$ is introduced into the system. The combined effect of the exchange coupling and anisotropy of the isolated SMM then open a significant gap, $f_{\mathrm{DTC}} = \sqrt{B^2 + \left(\frac{D}{2}\right)^2} - \frac{D}{2}$ in the energy spectrum when the SMM-array is placed in the periodic external field. This gap determines the DTC oscillation which is akin to the Rabi oscillations in interacting quantum many-body systems,[1] and quite surprisingly, even with increased $J$ remains unchanged. However, such 'many-body Rabi' oscillations are prone to destabilization unless specific conditions are met, such as Rydberg blockade in a Rydberg atom ensemble.[1] In our case, this necessary stabilization is provided by the $SU(2)$-symmetry of the exchange interactions. The dynamic involves transitions between the ground state and a coherent superposition of all single spin-flip states – a true manifestation of the many-body nature of the dynamics. Conversely, adopting Ising-type coupling, as we shall elaborate below, reveals a spectrum characterized by multiple similar-magnitude gaps, with the number of gaps increasing with the chain length, thereby introducing a noisy oscillation in the large (theoretically $N \to \infty$) Ising-coupled SMM chain and destroying the DTC.

We now demonstrate the above phenomenology on a more rigorous mathematical footing. We recognize that the Heisenberg coupling term in our system, represented by the formula:

$$-J \sum_j \mathbf{S}_j \cdot \mathbf{S}_{j+1}$$

is invariant under $SU(2)$ symmetry, i.e., this term remains unchanged under any rotation of the spin-space. This means that even if we change the orientation of our spin reference frame — for instance, by swapping $S_j^z \to -\tilde{S}_j^x$, and $S_j^x \to \tilde{S}_j^z$ — the form of our Hamiltonian

stays the same. Under this rotation of spin-space the new Floquet Hamiltonian looks like:

$$\mathcal{H}_F = -J \sum_j \tilde{\mathbf{S}}_j \cdot \tilde{\mathbf{S}}_{j+1} + \sum_j \left[ -D(\tilde{S}_j^x)^2 + B\tilde{S}_j^z \right].$$

Here, we note that the anisotropy term $D$ breaks the $SU(2)$ symmetry by making one direction in spin space energetically favorable, thus causing the magnetization vector to align along a specific plane, which in our case is the $XY$-plane. Therefore, in our rotated spin-space frame we define a dynamical symmetry operator, $\tilde{S}^+_{\text{tot}} = \sum_j \tilde{S}^+_j$, which exhibits what we call Larmor precession. Mathematically, this is represented as:

$$e^{iBt\tilde{S}^z_{\text{tot}}} \tilde{S}^+_{\text{tot}} e^{-iBt\tilde{S}^z_{\text{tot}}} = e^{iBt} \tilde{S}^+_{\text{tot}}.$$

Then, starting from an initial state $|\psi_0\rangle$ that breaks the symmetry, we observe persistent oscillations given by:

$$\begin{aligned} \langle\psi_0|e^{i\mathcal{H}_F t} \tilde{S}^+_{\text{tot}} e^{-i\mathcal{H}_F t}|\psi_0\rangle &\approx e^{iBt} \langle\psi_0|e^{-i\sum_j \left(J\tilde{\mathbf{S}}_j \cdot \tilde{\mathbf{S}}_{j+1} + D(\tilde{S}^x_j)^2\right)t} \tilde{S}^+_{\text{tot}} e^{i\sum_j \left(J\tilde{\mathbf{S}}_j \cdot \tilde{\mathbf{S}}_{j+1} + D(\tilde{S}^x_j)^2\right)t}|\psi_0\rangle \\ &\to c_0 e^{iBt}, \end{aligned} \tag{3}$$

where $c_0$ is a non-zero constant determined by the symmetry-broken initial state.[2] This mechanism is further corroborated by analyzing again Fig. 2, where four SMMs in an initial state configuration $\langle S^z_j \rangle = 1; 0; 1; 0$ end up behaving as a noisy oscillation, but a $1; 1; 1; 1$ configuration, being a fully aligned ferromagnetic state for $J > 0$, does not.

Below, we prove how $\tilde{S}^+_{\text{tot}} = \sum_j \tilde{S}^+_j$ is an approximate dynamical symmetry operator under the following conditions:

1. The amplitude of the external field must be much larger compared to the anisotropy, $B \gg D$.

2. The temperature is such that only low-lying excitations are present. This is true in

low temperatures and thermodynamic ($N \to \infty$) limit. Here the anisotropy term acts as a repulsive interaction between magnons when two magnons are brought nearby, cf. Ref 3, leading to the dissociation of any two-magnon bound state into a pair of one-magnon states. This is specific to the model we have considered, where the anisotropy and external field directions in the spin space are orthogonal to each other, and $(J,\ B) \gg D$.

3. The spin $S$ of the individual SMM must be large, especially compared to the number of spin flips appearing in the system, i.e., $S \gg n$.

To show the dynamical symmetry, we write $\mathcal{H}_F = \mathcal{H}_0 + \mathcal{H}_x$, where $\mathcal{H}_0 = -J\sum_j \tilde{\mathbf{S}}_j \cdot \tilde{\mathbf{S}}_{j+1} + \sum_j B\tilde{S}_j^z$, $\mathcal{H}_x = -\sum_j D(\tilde{S}_j^x)^2$. Clearly, the deviation of $\tilde{S}^+_{\text{tot}}$ being an exact dynamical symmetry is due to $[\mathcal{H}_x, \tilde{S}^+_{\text{tot}}] = -D\sum_j(\tilde{S}_j^x\tilde{S}_j^z + \tilde{S}_j^z\tilde{S}_j^x)$. However, following Ref. 3 we can show that in the limit $B \gg D$, large $S$, and low magnon density $\tilde{S}_j^+$ can be a dynamical symmetry.

We first note that when $B \gg D$ the term $\mathcal{H}_x$ can be treated as a perturbation to $\mathcal{H}_0$. The eigenstates of $\mathcal{H}_0$ corresponding to $\mathcal{H}_0|\psi_n\rangle = E_{0,n}|\psi_n\rangle$, are the ground state with $n = 0$, and magnons corresponding to all the other spin-flip states with the number of spin flipped being $n = 1, 2, \cdots$, and normalization $\langle\psi_m|\psi_n\rangle = \delta_{m,n}$.[3] More precisely, we consider the ground state to be $|\psi_0\rangle = |-S, -S, \cdots, -S, \cdots\rangle$ and the $n-$spin flipped state to be $|\psi_n\rangle = \sum_j |\cdots, (-S+n), \cdots\rangle$ at the bottom of the magnon dispersion with $\mathbf{k} = 0$.[3] The perturbation term,

$$\mathcal{H}_x = -\frac{D}{4}\sum_j \left(\tilde{S}_j^+\tilde{S}_j^+ + \tilde{S}_j^-\tilde{S}_j^- + \tilde{S}_j^+\tilde{S}_j^- + \tilde{S}_j^-\tilde{S}_j^+\right)$$

either couples the states differing by '0' spin-flips due to the term, $(\tilde{S}_j^-\tilde{S}_j^+ + \tilde{S}_j^+\tilde{S}_j^-) = S^2 - (\tilde{S}_j^z)^2$, or couples states that differ by two spin-flips on the same site due to $\tilde{S}_j^-\tilde{S}_j^- + \tilde{S}_j^+\tilde{S}_j^+$ term. The part of $\mathcal{H}_x$ connecting states differing by two spin flips at the same site gives second order correction and is given by, $\mathcal{H}^{(2)}_{\text{eff}} = \sum_n\sum_{m\neq n}\frac{|\langle\psi_m|\mathcal{H}_x|\psi_n\rangle|^2}{E_{0,m} - E_{0,n}}|\psi_n\rangle\langle\psi_n|$. The relevant denominator is the gap between any pair of states separated by two spin flips

$\Delta E_2 = E_{0,m+2} - E_{0,m} \approx 2B$ in the thermodynamic limit. We note on passing that for finite size systems the finite momentum magnon modes with $k = \frac{2\pi\ell}{N}$, with $-N \leq \ell \leq N$, will contribute and would make any analytical progress challenging. Therefore the second-order contribution becomes,

$$\begin{aligned}
\frac{|\langle\psi_{n+2}|\mathcal{H}_x|\psi_n\rangle|^2}{E_{0,n+2} - E_{0,n}} &= \frac{D^2}{16}\left[\frac{|\langle\psi_{n+2}|\sum_j(\tilde{S}_j^+\tilde{S}_j^+)|\psi_n\rangle|^2}{2B}\right] + \frac{D^2}{16}\left[\frac{|\langle\psi_n|\sum_j(\tilde{S}_j^-\tilde{S}_j^-)|\psi_{n+2}\rangle|^2}{2B}\right] \\
&= \frac{ND^2}{16B}\sqrt{(S(S+1))^2 - 2(S(S+1))(n+1)^2 + n(n+2)(n+1)^2} \\
&\approx \frac{ND^2}{16B}(S(S+1) - (n+1)^2) \\
&= \frac{ND^2}{16B}(S^2 - (n+1)^2) \text{ in the large} - S \text{ limit,}
\end{aligned} \tag{4}$$

where $\langle\psi_n|\psi_n\rangle = 1$ and $0 \leq n \leq 2S - 1$, and the factor $N$ comes from the fact that one can only have $N$ number of 2-spin-flip states in the system, one for each site. Furthermore, we note that $n = 2S, 2S + 1$ do not contribute to the second order correction because $\langle\psi_{n+2}|\sum_j(\tilde{S}_j^+\tilde{S}_j^+)|\psi_n\rangle = 0$ for these two values of $n$, and thus we can take the limit $0 \leq n \leq 2S+1$. Therefore, $\mathcal{H}_{\text{eff}}^{(2)} \approx \frac{ND^2}{16B}\sum_{n=0}^{2S+1}(S+n+1)(S-n-1)|\psi_n\rangle\langle\psi_n| \approx \frac{D^2(S+1)}{16B}\sum_{n=0}^{2S+1} N(S-n-1)|\psi_n\rangle\langle\psi_n| = \frac{(S+1)D^2}{16B}\sum_j \tilde{S}_j^z + \text{const.}$, where we have taken $(S+n+1) \approx S+1$ assuming a very low number of spin-deviations $n$ in the system with large–$S$, and the effective Floquet Hamiltonian is given by,

$$\mathcal{H}_{F,\text{eff}} \approx -J\sum_j \tilde{\mathbf{S}}_j \cdot \tilde{\mathbf{S}}_{j+1} + \sum_j \left(B + \frac{D}{4}\tilde{S}_j^z + \frac{(S+1)D^2}{16B}\right)\tilde{S}_j^z. \tag{5}$$

Here, although the number of spin-deviations $n$ can in principle range from 0 to $2S - 1$, in most of the physical conditions we can assume small values of $n$ so that the number of spin deviations occurring in the system is not appreciable. Note that to create any additional spin deviation on top of an $n-$spin-flipped ($n-$magnon) state at least an energy $\mathcal{O}(B)$ is necessary. For the above effective Hamiltonian $\tilde{S}_{\text{tot}}^+$ can be a dynamical symmetry if we

consider $(\tilde{S}_j^z)^2 \approx \langle \tilde{S}_j^z \rangle \tilde{S}_j^z = (-S + \frac{n}{N})\tilde{S}_j^z$ [1], i.e. a mean-field limit and the corresponding eigen-operator condition becomes,

$$[\mathcal{H}_{F,\mathrm{eff}}, \tilde{S}^+_{\mathrm{tot}}] = \left( B - \frac{D}{2}(S - \frac{n}{N}) + \frac{(S+1)D^2}{16B} \right) \tilde{S}^+_{\mathrm{tot}}. \tag{6}$$

Importantly, the dynamical symmetry eigenvalue depends on the number of spin-flips that appear in the system. Note that even in the second-order perturbation theory, we need large $S$ in the form of the mean-field limit otherwise (5) does not provide the dynamical symmetry condition.

Eq. (6) corroborates our numerical findings. When the temperature is low, and the system only the low-lying excitations, i.e., $n \ll N$, eq. (6) shows that for $S = 1$ case, the eigenvalue corresponding to the dynamical-symmetry is given by $B - \frac{D}{2} + \frac{D^2}{8B}$. Put simply, $f_{DTC} = \sqrt{B^2 + \frac{D^2}{4}} - \frac{D}{2} \approx B - \frac{D}{2} + \frac{D^2}{8B}$ in the $B \gg D$ limit for $n \leq 1$ is the eigenvalue of the dynamical symmetry eigen-operator condition, as numerically obtained in the main text. Rotating back the spin-space the dynamical symmetry operator is $\tilde{S}^+_{tot} = \sum_j \left( S_j^z + i S_j^y \right)$, showing overlap with the magnetization, and $\mathfrak{Re}(\tilde{S}_j^+)$ shows DTC oscillation.

To further corroborate our phenomenology – a dynamical symmetry is approximately satisfied in the low-temperature when only low-lying excitations are excited in the system and $B \gg D$, we plot in Fig. 5(a) the dynamical symmetry eigenvalue as a function of spin$-S$ and $N = 3$ and compare that of the numerical results we reported in Fig. 4(b) of the main text. Fig. 5(a) perfectly matches analytical and numerical results with a maximum error of 0.5% only. Furthermore, Fig. 5(b) plots the DTC oscillation amplitude as a function of time on a log-scale for $N = 3 - 7$. The black arrow indicates that the amplitude remains finite for a longer time as we increase the chain length $N$ from 3 to 7. This hints that the oscillation would indeed survive for a long time (hence pre-thermal) in the limit $N \to \infty$

[1] For each site the eigenvalues of $\tilde{S}_j^z$ ranges from $-S$ to $S$. Since the $n$ spin-flip state $|\psi_n\rangle \sim \sum_j | \cdots, (-S+n), \cdots \rangle$ with a suitable normalization factor, for an $N$-site chain the average contribution of the total $n$ spin-flips to one site is, therefore, $n/N$.

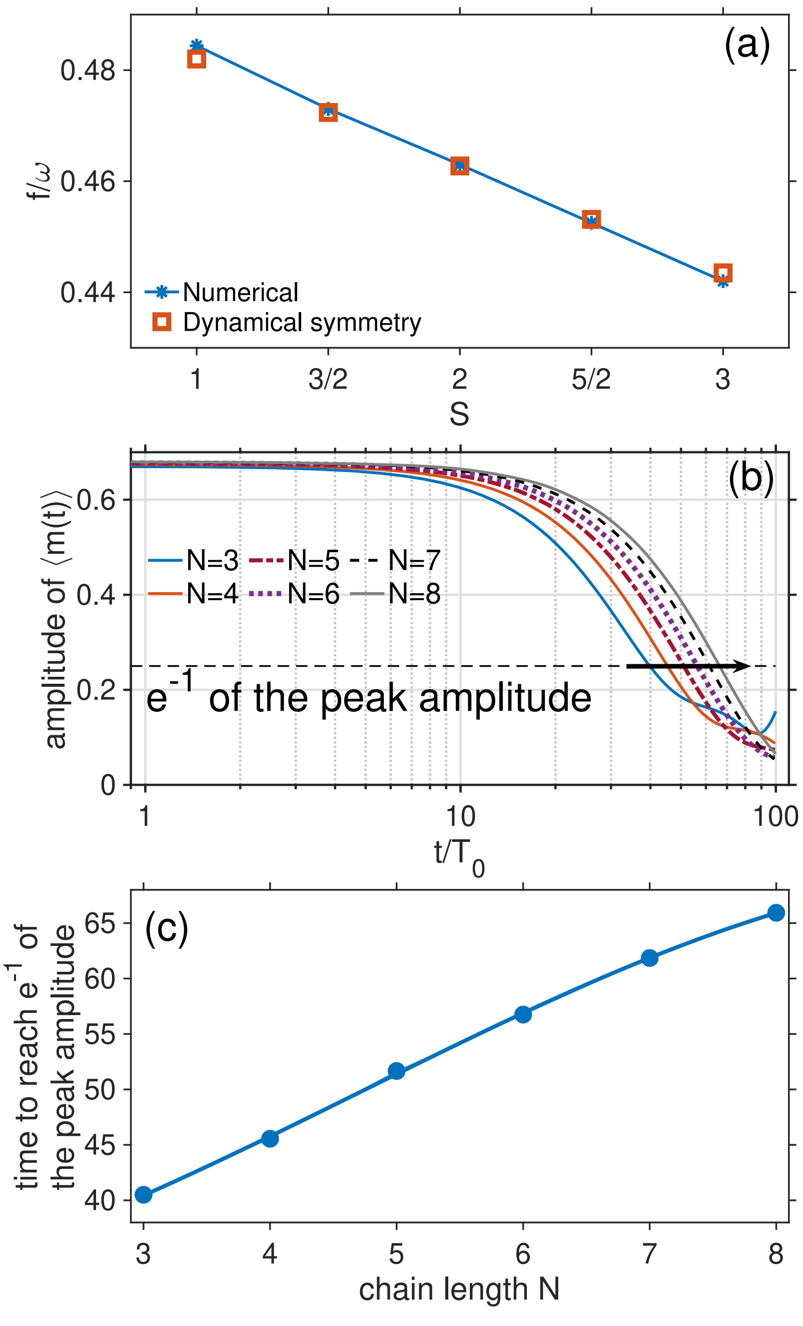


Figure 5: (a) Plot of numerically obtained (for $N = 3$) $f/\omega$ (blue line) and the dynamical symmetry eigenvalue $\left(B - \frac{D}{2}(S - \frac{n}{N}) + \frac{(S+1)D^2}{16B}\right)$ (orange dashed line) as a function of $S$ with $n = 1$ and $N = 3$ in the latter. The numerical data corresponds to Fig. 4(b) blue dots of the main text. (b) Plot of the DTC oscillation amplitude as a function of time on a log scale for $N = 3 - 7$. The black arrow indicates the direction of increasing amplitude. (c) Plot of the time $\tau/T_0$ to reach $e^{-1}$ of the peak value of the amplitude of the DTC oscillation.

before its decay.

In Fig. 5(c), we show the relationship between the chain length $N$ and the time $\tau/T_0$ required for the amplitude of the DTC oscillation to decay by $1/e$ of the peak amplitude. As the chain length $N$ increases, the time $\tau/T_0$ also increases, indicating that longer chains stabilize the DTC oscillations for a longer duration before decaying. The hint of saturation of this time scale at very large $N$ values further suggests that the oscillation would remain stable for a long time before eventually decaying.

An example case where a different coupling between the SMMs would alter the outcome is the Ising coupling. In this case, the Floquet Hamiltonian is given by, $\mathcal{H}_F = -J \sum_j S_j^z S_{j+1}^z + \sum_j \left[-D(S_j^z)^2 + BS_j^x\right]$. We adopt the same parameters as used in the main text, $J = 10D$, $\omega = 2\pi D$, and $B = \omega/2$. Fig. 6 compares DFT $\Phi\left[\langle S_1^z(t)\rangle\right](f)$ of the on-site magnetization for three system sizes, $N = 3, 4, 5$. In this case, the number of sub-harmonic peaks increases as the system size increases. This trend suggests that enlarging the system size results in the emergence of additional subharmonic frequencies, culminating in an infinite array of such frequencies in the limit as $N \to \infty$, thereby destabilizing the DTC. Physically, this phenomenon can be attributed to the gapped nature of the many-body spectrum in finite-sized systems with $Z_2$ symmetry, where the most significant energy gap spans across the spectrum rather than being localized in a portion of the many-body spectrum. Consequently, transitions occur through multiple gaps, giving rise to numerous sub-harmonic frequencies.

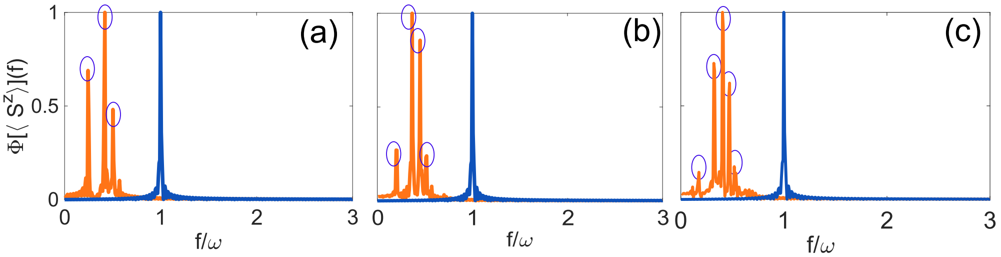


Figure 6: Plot of discrete Fourier transform $\Phi\left[\langle S_1^z(t)\rangle\right](f)$ of the on-site magnetization in an Ising-coupled SMM-chain as a function of frequency $f/\omega$ for different system-sizes, (a) $N = 3$, (b) $N = 4$, and (c) $N = 5$. The sub-harmonic peaks are encircled.

## Condition for sub-harmonic response

In Fig. 7 we show how the sub-harmonic response depends on the magnitude $B$ of the external field relative to its frequency $\omega$. The figure presents Discrete Fourier Transform (DFT) plots of onsite magnetization $\Phi[\langle S_j^\alpha(t)\rangle](f)$ as a function of $f/\omega$. It distinguishes between two distinct scenarios: (a) when $B > \omega$ $(= 2\omega)$, characterized as the higher-harmonic case, and (b) when $B < 0$ $(= 0.5\omega)$, considered as the sub-harmonic case. Notably, the higher-harmonic response appears in $B > \omega$ $(= 2\omega)$ in the $x-$component of the on-site magnetization as highlighted.

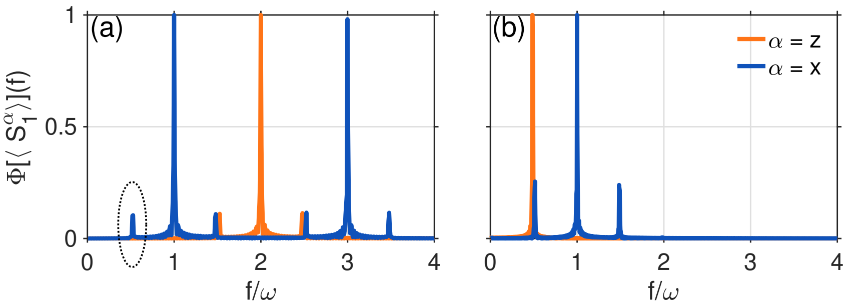


Figure 7: Plots of DFT of onsite magnetization $\Phi[\langle S_j^\alpha(t)\rangle](f)$ as a function of $f/\omega$ for (a) $B > \omega$ $(= 2\omega)$ the higher-harmonic case, and (b) $B < 0$ $(= 0.5\omega)$ the sub-harmonic case. The sub-harmonic response corresponds to $B > \omega$ $(= 2\omega)$ in the $x-$component of the on-site magnetization is encircled.

## References

(1) Dudin, Y.; Li, L.; Bariani, F.; Kuzmich, A. Observation of coherent many-body Rabi oscillations. *Nature Physics* **2012**, *8*, 790–794.

(2) Khemani, V.; Moessner, R.; Sondhi, S. L. A Brief History of Time Crystals. *arXiv preprint arXiv:1910.10745* **2019**, Submitted on 23rd October 2019.

(3) Chauhan, P.; Mahmood, F.; Changlani, H. J.; Koohpayeh, S. M.; Armitage, N. P. Tunable Magnon Interactions in a Ferromagnetic Spin-1 Chain. *Phys. Rev. Lett.* **2020**, *124*, 037203, Publisher: American Physical Society.
